# Supplementary material for: Coordinate Descent for Network Linearization
Source: arXiv:2511.11781 source file (2025-11-14)
Supplement: Supplementary file 1 [file 00999_autorep.tex]

\paragraph{AutoReP Hysteresis as Truncated Gradients:}
% \shai{One of the contributions of AutoReP is the use of hystersis to improve convergence... We show that this procedure is rooted in truncated gradients methods.}
When the budget fails to decrease by some differential budget, SNL increases the Lagrange Multiplier by some constant. This masks out a bulk of ReLUs and turns-on the mask for others. To compensate for the abrupt changes in mask values across the optimization stage, AutoRep~\cite{peng2023autorep} suggests a hysteresis mechanism which stabilizes the binarized ReLU replacement training process. This is formally stated in Equation~\ref{eq:autorep_hysteresis_eq} and visualized in figure~\ref{fig:autorep_hysteresis}. 
{\small
\begin{equation}\label{eq:autorep_hysteresis_eq}
m_{i\: k, t+1} =  \left \{ \begin{array}{cccc}
1,  &\textnormal{$m_{i\: k, t} = 1$ and $m_{W, i\: k} > -t_h$} \\
0,  &\textnormal{$m_{i\: k, t} = 1$ and $m_{W, i\: k} \leq -t_h$} \\
0,  &\textnormal{$m_{i\: k, t} = 0$ and $m_{W, i\: k} \leq t_h$} \\
1,  &\textnormal{$m_{i\: k, t} = 0$ and $m_{W, i\: k} > t_h$}\\
\end{array} \right.
\end{equation}
}
% \begin{figure}[t]
%     \centering
%       % \includegraphics[width=0.95\linewidth]{Fig/Forward.pdf}
%       \includegraphics[width=0.8\linewidth]{icml2024/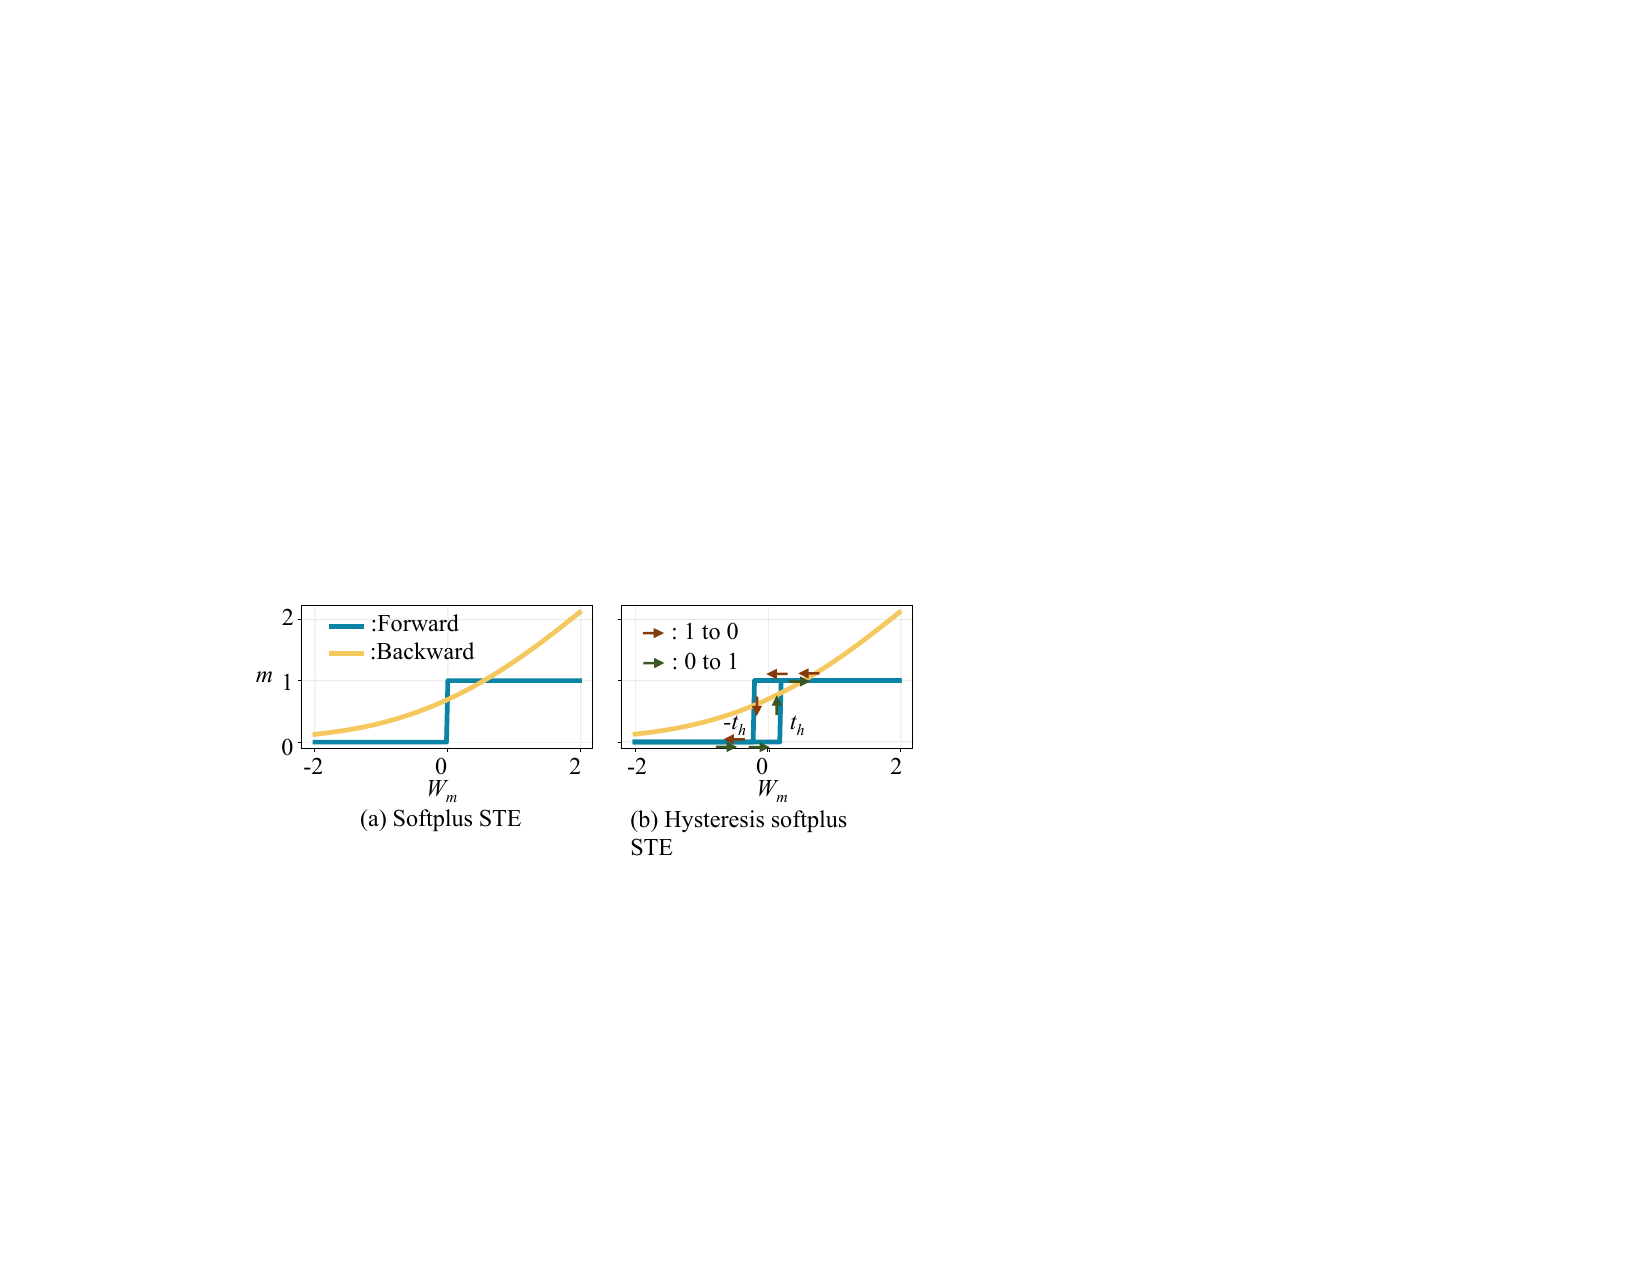}
%   \caption{AutoRep's Hysteresis indicator parameter update. }
%     \label{fig:autorep_hysteresis}
% \end{figure}
\begin{figure}
    \centering
    \resizebox{0.98\linewidth}{!}{
    \input{tikz/autoreps_hysteresis}
    }
    \caption{\textbf{AutoRep's Hysteresis which aims at mask values stabilization:} Truncated Gradients~\cite{langford2009sparse} shrink the coefficient to zero by a smaller amount and AutoRep~\cite{peng2023autorep} reduces the possibility of the indicator flip through the suggested hysteresis structure of the indicator value.}
     \label{fig:autorep_hysteresis}
\end{figure}

We show that this procedure is rooted in truncated gradients methods~\cite{langford2009sparse}. Both methods address the aggressive procedure of thresholding the optimization step result. Truncated gradients shrink the coefficient to zero by a smaller amount and AutoRep reduces the possibility of the indicator flip through their suggested hysteresis structure of the indicator value.
