# Supplementary material for: Coordinate Descent for Network Linearization
Source: arXiv:2511.11781 source file (2025-11-14)
Supplement: Supplementary file 2 [file 07_ours_on_top_of_autorep.tex]

\subsection{AutoRep ResNet18 Hyperparameters}
In this setting, we use a DRC of 80, ADT of 0.3\%, up to 50 RTs and 20 finetune epochs. We follow AutoRep and modify our optimizer to ADAM with an initial learning rate of $3.5\cdot 10^{-5}$ and a cosine annealing scheduler.

\subsection{AutoRep WideResNet Hyperparameters}
TBD
